# Supplementary material for: BeamScatter: Scalable, Deployable Long-Range backscatter communication with Beam-Steering
Source: arXiv:2110.14585 source file (2022-10-14)
Supplement: Supplementary file 1 [file Appendix.tex]

% !TEX root = main.tex

\section{Appendix} \label{appendix}
